# Supplementary material for: Path-Based Attention Neural Model for Fine-Grained Entity Typing
Source: arXiv:1710.10585 source file (2018-01-09)
Supplement: Supplementary file 1 [file supplementary.pdf]

# Path-Based Attention Neural Model for Fine-Grained Entity Typing

Denghui Zhang<sup>1</sup>, Pengshan Cai<sup>2</sup>, Yantao Jia<sup>1</sup>, Manling Li<sup>1</sup>, Yuanzhuo Wang<sup>1</sup>

<sup>1</sup>Institute of Computing Technology, Chinese Academy of Sciences, Beijing, 100190, China

<sup>2</sup>School of Computer Science University of Massachusetts Amherst Amherst, MA 01003

zhangdenghui@ict.ac.cn, pengshancai@cs.umass.edu, jamaths.h, limanlingcs@gmail.com, wangyuanzhuo@ict.ac.cn

## Abstract

Fine-grained entity typing aims to assign entity mentions in the free text with types (e.g., person, politician, etc.), which are arranged in a hierarchical structure. Traditional distant supervision based methods employ a structured data source as a weak supervision and do not need hand-labeled data, but they neglect the label noise in the automatically labeled training corpus. Although recent studies prune wrong data ahead of training, they suffer from error propagation and bring much parameter and computation complexity. In this paper, we propose an end-to-end typing model, called the path-based attention neural model (PAN) by leveraging the hierarchical structure of types to learn a noise-robust performance. Experiments on two data sets demonstrate its effectiveness.

## Introduction

Fine-grained entity typing aims to assign types to entity mentions in the local context (a single sentence), and the type set constitutes a tree-structured hierarchy, called type hierarchy. Recent years witness the boost of neural models in this task, e.g., (Shimaoka et al. 2016) employs an attention LSTM to attain sentence representations and achieves state-of-the-art performance. However, it still suffers from noise in training data, which is a main challenge in this task. The training data is generated by distant supervision, which assumes that if an entity has a type in knowledge bases (KBs), then all sentences containing this entity will express this type. Specifically, the process of generating training data by distant supervision is illustrated in Figure 1. Firstly the entity mentions are extracted from sentences. Then, the mentions are linked to entities in KB by entity linking techniques. Finally the type set of the respective entity is assigned to entity mentions and the training data is automatically generated. It avoids high expense of hand labeled data, but it will inevitably introduce irrelevant types to the context. For example, the entity “Donald Trump” has types “person”, “businessman” and “politician” in KBs, thus all three types are annotated for its mentions in the training corpora. But in sentence “Donald Trump announced his candidacy for President of US.”, only “person” and “politician” are correct types, while “businessman” can not be deduced from the sentence, so serves as noise. To alleviate this issue, a few

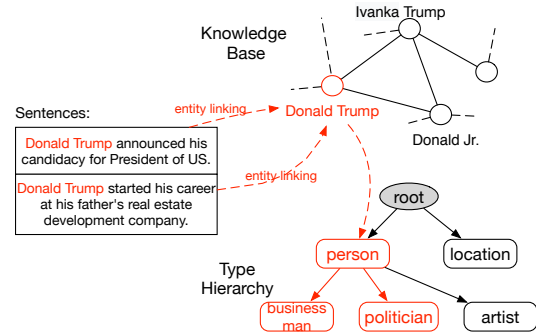

Figure 1: The distant supervision procedure to generate training data of “Donald Trump”.

systems try to denoise training data by filtering irrelevant types ahead of training. For instance, (Ren et al. 2016) proposes PLE, an embedding method to identify correct types for each mention, then use clean data to train classifiers. However, the denoising and training process are not unified, which may cause error propagation and bring much computation and parameter complexity.

Motivated by this, we propose an end-to-end typing model, called the path-based attention neural model (PAN), to focus on relevant sentences to each type, which can dynamically reduce the weights of wrong labeled sentences for each type during training. This idea is inspired by some successful attempts to reduce noise in relation extraction, e.g., (Lin et al. 2016). However, these methods fails to formulate type hierarchy, which is distinct in fine-grained entity typing. Specifically, if a sentence indicates a type, its parent type can be also deduced from the sentence. Like the example above, “politician” is the subtype of “person”. Since the sentence indicates that “Donald Trump” is “politician”, “person” should also be assigned. Considering this hierarchical constraint, path-based attention for each type is obtained based on its path to the top coarse type (e.g., “person”, “businessman”) in type hierarchy, which enables parameter sharing of types in the same path, and thus reduce noise effectively and yields a better typing classifier. Experiments validate effectiveness of PAN.

## Related Work

Fine-grained entity typing aims to assign entity mentions with a much larger set of fine-grained types (Ling and Weld 2012), and has been paid great attention recent years. Unlike coarse types (e.g., person, location), this task can not be tackled by multi-class classification following the type mutual exclusion assumption (i.e., one type per mention). Actually, it is formulated as multi-label multi-class(hierarchical) classification problems.

A main challenge in fine-grained entity typing is the absence of annotated data, and the training data is generated by distant supervision, which use a knowledge base to generate possible types, and will inevitably introduce label noise. This problem is first discussed by (Gillick et al. 2014), which also introduces the concept of context-dependent fine-grained entity typing, where the types of a mention is constrained to what can be deduced from its context. In order to encourage more research on the problem, they introduce a new OntoNotes-derived manually annotated evaluation dataset. In addition, they proposed three label cleaning heuristics to reduce the label noise. More recently, (Ren et al. 2016) proposed a heterogeneous partial-label embedding framework to denoise the data. It removes false positives and leaves only the correct ones for each mention based on its local context.

Similar noise issue has also been encountered in relation extraction task, and the noise induced by distant supervision limit the accuracy of relation prediction. Relation extraction problem can be formulated as a multi-label problem, and MultiR(Hoffmann et al. 2011) try to denoise the training data by selecting the most relevant sentence for each label while training. (Lin et al. 2016) proposed a selective attention model to learn attention weights to score how well a sentence matches the relation and uses the weights to sum the sentences. It can avoid losing too much information and de-emphasize irrelevant sentences.

Inspired by their work, we propose our end-to-end path-based attention neural model to tackle the noise issue in fine-grained entity typing. We extend their model to a multi-label version, and then use the representation of paths to model the attention of each type, which can leverage hierarchical structure to reduce noise. As far as we know, we are the first to combine hierarchical information with attention to learn a noise-robust performance in fine-grained entity typing.

## Path-Based Attention Neural Model

The architecture of PAN is shown in Figure2. Supposing that there are  $n$  sentences containing entity  $e$ , i.e.,  $\mathcal{S}_e = \{s_1, s_2, \dots, s_n\}$ , and  $\mathcal{T}_e$  is the automatically labeled types based on KBs. Firstly PAN employs LSTM to generate representations of sentences  $s_i$  following (Shimaoka et al. 2016), where  $s_i \in \mathbb{R}^d$  is the representation of  $s_i$ ,  $i \in \{1, 2, \dots, n\}$ . Afterwards, we build path-based attention  $\alpha_{i,t}$  over sentences  $s_i$  for each type  $t \in \mathcal{T}_e$ , which is expected to focus on relevant sentences to  $t$ . Then, the representation of sentence set  $\mathcal{S}_e$  for  $t$ , denoted by  $s_{e,t} \in \mathbb{R}^d$ , is calculated through weighted sum of vectors of sentences. Finally, we obtain predicted types through a classification layer.

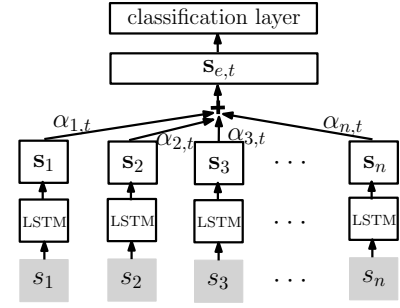

Figure 2: The architecture of PAN for given entity  $e$ , type  $t$

More precisely, given  $e$ , an attention  $\alpha_{i,t}$  is learned to score how well sentence  $s_i$  matches type  $t$ , i.e.,

$$\alpha_{i,t} = \frac{\exp(s_i \mathbf{A} \mathbf{p}_t)}{\sum_{j=1}^n \exp(s_j \mathbf{A} \mathbf{p}_t)},$$

where  $\mathbf{A} \in \mathbb{R}^{d \times d}$  is a weighted diagonal matrix.  $s_i \in \mathbb{R}^d$  is generated through an LSTM based neural model, and its architecture is illustrated in Figure3. Its input is the entity mention and context, and the output is the concatenation of entity mention representation and the context representation.

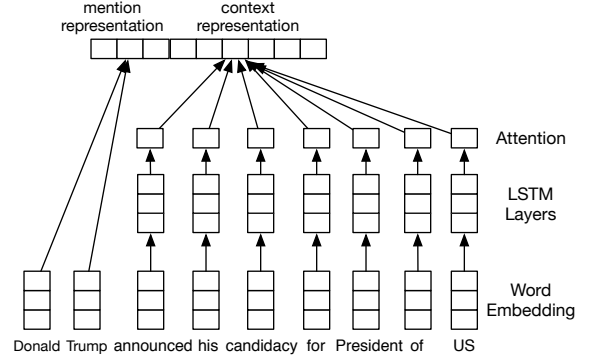

Figure 3: The distant supervision procedure to generate training data of "Donald Trump".

In addition,  $\mathbf{p}_t \in \mathbb{R}^d$  is the representation of path  $p_t$  for type  $t$ . Specifically, for each type, we define one path as a sequence of types starting from its top coarse type, and ending with it. More formally, for type  $t_l$ ,  $p_{t_l} = t_1 \rightarrow t_2 \rightarrow \dots \rightarrow t_l$ , where  $t_1$  is its respective top coarse type, and  $t_{i+1}$  is the subtype of  $t_i$ . For example, according to the type hierarchy in Figure1, for type  $t_l = \text{politician}$ , its path is  $p_{t_l} = \text{person} \rightarrow \text{politician}$ .

We represent the path  $p_{t_l}$  as a semantic composition of all relevant entity types, i.e.,

$$\mathbf{p}_{t_l} = \mathbf{t}_1 \circ \mathbf{t}_2 \circ \dots \circ \mathbf{t}_l,$$

where  $\mathbf{t}_i \in \mathbb{R}^d$  is the representation of type  $t_i$ , which is a parameter to learn.  $\circ$  is a composition operator. In this paper, we consider two types of operators: (1) Addition (PAN-A), where  $\mathbf{p}_{t_l}$  equals the sum of type vectors, i.e.,

$$\mathbf{p}_{t_l} = \mathbf{t}_1 + \mathbf{t}_2 + \dots + \mathbf{t}_l.$$

(2) Multiplication (PAN-M), where  $\mathbf{p}_{t_l}$  equals the cumulative product of type vectors, i.e.,

$$\mathbf{p}_{t_l} = \mathbf{t}_1 \cdot \mathbf{t}_2 \cdot \dots \cdot \mathbf{t}_l.$$

In this way, path-based attention enables the model to share parameters between types in the same path. For example, the attention learned for “person” could assist the learning of the attention for “politician”. It makes learning easier especially for infrequent subtypes, which suffer from dearth of training data, since the attentions for these subtypes can get support from the attention for parent type.

Then, the representation of sentence set  $\mathcal{S}_e$  for type  $t$ , i.e.,  $\mathbf{s}_{e,t}$ , is calculated through weighted sum of sentence vectors,

$$\mathbf{s}_{e,t} = \sum_{i=1}^n \alpha_{i,t} \mathbf{s}_i.$$

Since one mention can have multiple types, we employ a classification layer consisting of  $N$  logistic classifiers, where  $N$  is the total number of types. Each classifier outputs the probability of respective type, i.e.,

$$P(t|\mathbf{s}_{e,t}) = \frac{\exp(\mathbf{w}_t^T \mathbf{s}_{e,t} + \mathbf{b}_t)}{1 + \exp(\mathbf{w}_t^T \mathbf{s}_{e,t} + \mathbf{b}_t)},$$

where  $\mathbf{w}_t, \mathbf{b}_t \in \mathbb{R}^d$  are the logistic regression parameters. To optimize the model, a multi-type loss is defined according to the cross entropy as follows,

$$J = - \sum_e \sum_t [\mathbb{I}_t \ln P(t|\mathbf{s}_{e,t}) + (1 - \mathbb{I}_t) \ln(1 - P(t|\mathbf{s}_{e,t}))],$$

where  $\mathbb{I}_t$  is indicator function to indicate whether  $t$  is the annotated type of entity  $e$ , i.e.,  $t \in \mathcal{T}_e$ .

## Experiments

Experiments are carried on two widely used datasets OntoNotes and FIGER(GOLD), and the training dataset of OntoNotes is noisy compared to FIGER(GOLD) according to (Shimaoka et al. 2016). The statistics of the datasets are listed in Table 1. During training process, we use “raw” noisy data provided by (Shimaoka et al. 2016).

Table 1: Statistics of the datasets.

| Datasets    | #Type | #Layer | #Context | #Train | #Test |
|-------------|-------|--------|----------|--------|-------|
| OntoNotes   | 89    | 3      | 143K     | 223K   | 8,963 |
| FIGER(GOLD) | 113   | 2      | 1.51M    | 2.69M  | 563   |

We employ Strict Accuracy (Acc), Loose Macro F1 (Ma-F1), and Loose Micro F1 (Mi-F1) as evaluation measures following (Shimaoka et al. 2016) and Ren2016Label. Specifically, let  $T$  denote evaluation set. For each mention  $m \in T$ , we denote its ground-truth types as  $t_m$  and the predicted types as  $\bar{t}_m$ .

- Strict: The prediction is considered correct if and only if  $t_m = \bar{t}_m$ :

$$Accuracy(\mathbf{Acc}) = \sum_{m \in T} \mathbb{I}\{t_m = \bar{t}_m\} / |T|$$

- Loose Macro: The Macro-Precision (Ma-P) and MacroRecall (Ma-R) are computed for each mention, then their F1 is computed.

$$\mathbf{Ma-P} = \frac{1}{|T|} \sum_{m \in T} |t_m \cap \bar{t}_m| / |\bar{t}_m|$$

$$\mathbf{Ma-R} = \frac{1}{|T|} \sum_{m \in T} |t_m \cap \bar{t}_m| / |t_m|$$

$$\mathbf{Ma-F1} = \frac{2 * \mathbf{Ma-P} * \mathbf{Ma-R}}{\mathbf{Ma-P} + \mathbf{Ma-R}}$$

- Loose Micro: The Micro-Precision (Mi-P) and MicroRecall (Mi-R) scores are averages over all mentions, then their F1 is computed.

$$\mathbf{Mi-P} = \frac{\sum_{m \in T} |t_m \cap \bar{t}_m|}{\sum_{m \in T} |\bar{t}_m|}$$

$$\mathbf{Mi-R} = \frac{\sum_{m \in T} |t_m \cap \bar{t}_m|}{\sum_{m \in T} |t_m|}$$

$$\mathbf{Mi-F1} = \frac{2 * \mathbf{Mi-P} * \mathbf{Mi-R}}{\mathbf{Mi-P} + \mathbf{Mi-R}}$$

The baselines are chosen from two aspects: (1) Predicting types in a unified process using raw noisy data, i.e., HYENA (Yosef et al. 2012), FIGER (Ling and Weld 2012) and TLSTM (Shimaoka et al. 2016). (2) Predicting types using clean data by denoising ahead, i.e., H\_PLE and F\_PLE (Ren et al. 2016). To prove the superiority of considering hierarchy, we also directly apply the attention neural model in relation extraction (Lin et al. 2016) without considering type hierarchy (AN). We obtain the optimal hyperparameters from preliminary experiments by evaluating model performance on the development sets. Concretely, the hidden-size of the LSTM was set to 100, and we used Adam as our optimisation method with a learning rate of 0.001, a mini-batch size of 1000. In order to make a fair comparison between the performance of our path-based attention mechanism and the neural architecture of (Shimaoka et al. 2016), we use the same word embeddings to represent sentence as they use. Our model implementation was done in Python using the Pytorch machine learning library. The results of baselines are the best results reported in their papers.

Table 2: Performance on FIGER(GOLD) and OntoNotes

| Metric | OntoNotes   |             |             | FIGER(GOLD) |             |             |
|--------|-------------|-------------|-------------|-------------|-------------|-------------|
|        | Acc         | Ma-F1       | Mi-F1       | Acc         | Ma-F1       | Mi-F1       |
| HYENA  | 24.9        | 49.7        | 44.6        | 28.8        | 52.8        | 50.6        |
| FIGER  | 36.9        | 57.8        | 51.6        | 47.4        | 69.2        | 65.5        |
| TLSTM  | 50.8        | 70.1        | 64.9        | 59.7        | 79.0        | 75.4        |
| AN     | 52.3        | 71.7        | 65.2        | 60.0        | 79.5        | 75.9        |
| PAN-A  | <b>54.9</b> | <b>72.8</b> | <b>66.5</b> | <b>60.2</b> | <b>79.9</b> | <b>76.2</b> |
| PAN-M  | 53.0        | 71.9        | 65.3        | 60.0        | 79.4        | 76.0        |

We can observed from Table2 that:

(1) When using the same raw noisy data, PAN outperforms all methods on both data sets. TLSTM achieves the best performance among baselines, while PAN-A improve 4% in Strict Accuracy, which is the most sensitive measure

to noise and the most difficult one to enhance. Thus, it proves the anti-noise ability of PAN.

(2) PAN performs better than AN, it can be easily understood that the attention learned in PAN utilizes the hierarchical structure to enable parameter sharing, therefore, the type hierarchy can help to enhance the typing performance.

(3) The improvements on OntoNotes are higher than FIGER(GOLD), because OntoNotes is more noisy, and the hierarchical structure in OntoNotes is more complex with more layers, which further demonstrates that path-based attention does well with type hierarchy, and proves the superiority of PAN in reducing noise for data sets with more noise.

(4) PAN-A achieves better performance than PAN-M, which shows that addition operator can better capture type hierarchy.

Table 3: Performance on FIGER(GOLD) and OntoNotes

| Metric | OntoNotes   |             |             | FIGER(GOLD) |             |             |
|--------|-------------|-------------|-------------|-------------|-------------|-------------|
|        | Acc         | Ma-F1       | Mi-F1       | Acc         | Ma-F1       | Mi-F1       |
| H_PLE  | 54.6        | 69.2        | 62.5        | 54.3        | 69.5        | 68.1        |
| F_PLE  | <b>57.2</b> | 71.5        | 66.1        | 59.9        | 76.3        | 74.9        |
| PAN-A  | 54.9        | <b>72.8</b> | <b>66.5</b> | <b>60.2</b> | <b>79.9</b> | <b>76.2</b> |

As shown in Table3, PAN achieves comparable performance on Acc by using raw noisy data with H\_PLE and F\_PLE using denoised training data, and PAN even has higher Ma-F1 and Mi-F1. It makes sense that PLE has higher Acc on OntoNotes since the noise is reduced before training, but considering the efficiency, PAN is an end-to-end process without bringing much complexity, thus is more effective to reduce noise.

## Conclusion and Future Work

In conclusion, PAN can reduce noise through an end-to-end process, and thus can achieve better typing performance without bring much complexity. Moreover, it performs better on the dataset with more noise and more complex hierarchy.

In the future, we will explore the formulation of path representations, such as using RNN or other operators to better capture the hierarchical constraints between types. Besides, we also think that we can better model the classification layer by considering type hierarchy, which may help to utilize the hierarchical structure more thoroughly.

## References

Gillick, D.; Lazic, N.; Ganchev, K.; Kirchner, J.; and Huynh, D. 2014. Context-dependent fine-grained entity type tagging. *arXiv preprint arXiv:1412.1820*.

Hoffmann, R.; Zhang, C.; Ling, X.; Zettlemoyer, L.; and Weld, D. S. 2011. Knowledge-based weak supervision for information extraction of overlapping relations. In *Proceedings of the 49th Annual Meeting of the Association for Computational Linguistics: Human Language Technologies-Volume 1*, 541–550. Association for Computational Linguistics.

Lin, Y.; Shen, S.; Liu, Z.; and et al. 2016. Neural relation extraction with selective attention over instances. In *ACL*.

Ling, X., and Weld, D. S. 2012. Fine-grained entity recognition. In *AAAI*.

Ren, X.; He, W.; Qu, M.; Voss, C. R.; Ji, H.; and Han, J. 2016. Label noise reduction in entity typing by heterogeneous partial-label embedding. In *KDD*.

Shimaoka, S.; Stenetorp, P.; Inui, K.; and Riedel, S. 2016. Neural architectures for fine-grained entity type classification. In *EACL*.

Yosef, M. A.; Bauer, S.; Hoffart, J.; Spaniol, M.; and Weikum, G. 2012. Hyena: Hierarchical type classification for entity names.
