# Supplementary material for: Path-Based Attention Neural Model for Fine-Grained Entity Typing
Source: arXiv:1710.10585 source file (2018-01-09)
Supplement: Supplementary file 2 [file supplenew.pdf]

# Path-Based Attention Neural Model for Fine-Grained Entity Typing

Denghui Zhang<sup>1</sup>, Pengshan Cai<sup>2</sup>, Yantao Jia<sup>1</sup>, Manling Li<sup>1</sup>, Yuanzhuo Wang<sup>1</sup>

<sup>1</sup>Institute of Computing Technology, Chinese Academy of Sciences, Beijing, 100190, China

<sup>2</sup>School of Computer Science University of Massachusetts Amherst Amherst, MA 01003

zhangdenghui@ict.ac.cn, pengshancai@cs.umass.edu, jamaths.h, limanlingcs@gmail.com, wangyuanzhuo@ict.ac.cn

## Abstract

Fine-grained entity typing aims to assign entity mentions in the free text with types arranged in a hierarchical structure. Traditional distant supervision based methods employ a structured data source as a weak supervision and do not need hand-labeled data, but they neglect the label noise in the automatically labeled training corpus. Although recent studies use many features to prune wrong data ahead of training, they suffer from error propagation and bring much complexity. In this paper, we propose an end-to-end typing model, called the path-based attention neural model (PAN) by leveraging the hierarchical structure of types to learn a noise-robust performance. Experiments demonstrate its effectiveness.

## Introduction

Fine-grained entity typing aims to assign types (e.g., “person”, “politician”, etc.) to entity mentions in the local context (a single sentence), and the type set constitutes a tree-structured hierarchy (i.e., type hierarchy). Recent years witness the boost of neural models in this task, e.g., (Shimaoka et al. 2016) employs an attention based LSTM to attain sentence representations and achieves state-of-the-art performance. However, it still suffers from noise in training data, which is a main challenge in this task. The training data is generated by distant supervision, which assumes that if an entity has a type in knowledge bases (KBs), then all sentences containing this entity will express this type. Specifically, the process of generating training data by distant supervision is illustrated in Figure 1. Firstly the entity mentions are extracted from sentences. Then, the mentions are linked to entities in KB by entity linking techniques. Finally the type set of the respective entity is assigned to entity mentions and the training data is automatically generated. It avoids high expense of hand labeled data, but it will inevitably introduces irrelevant types to the context. For example, the entity “Donald Trump” has types “person”, “businessman” and “politician” in KBs, thus all three types are annotated for its mentions in the training corpora. But in sentence “Donald Trump announced his candidacy for President of US.”, only “person” and “politician” are correct types, while “businessman” can not be deduced from the sentence, thus serves as

noise. To alleviate this issue, a few systems try to denoise training data by filtering irrelevant types ahead of training. For instance, (Ren et al. 2016) proposes PLE to identify correct types by jointly embedding mentions, context and type hierarchy, and then use clean data to train classifiers. However, the denoising and training process are not unified, which may cause error propagation and bring much additional complexity.

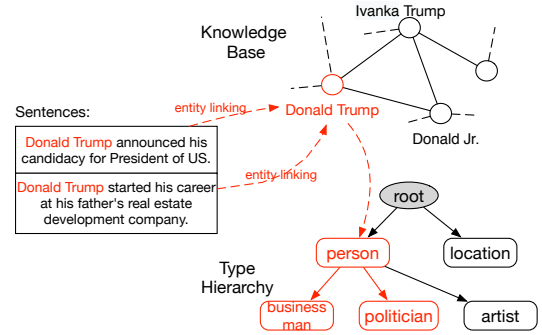

Figure 1: The distant supervision procedure to generate training data of “Donald Trump”.

Motivated by this, we propose an end-to-end typing model, called the path-based attention neural model (PAN), to focus on relevant sentences to each type, which can dynamically reduce the weights of wrong labeled sentences for each type during training. This idea is inspired by some successful attempts to reduce noise in relation extraction, e.g., (Lin et al. 2016). However, these methods fail to formulate type hierarchy, which is distinct in fine-grained entity typing. Specifically, if a sentence indicates a type, its parent type can be also deduced from the sentence. Like the example above, “politician” is the subtype of “person”. Since the sentence indicates that “Donald Trump” is “politician”, “person” should also be assigned. Thus, we build path-based attention for each type by utilizing its path to its coarsest parent type (e.g., person, businessman) in the type hierarchy. Compared to the simple attention in relation extraction, it enables parameter sharing for types in the same path. With the support of hierarchical information of types, it can reduce noise effectively and yields a better typing classifier. Experiments on two data sets validate effectiveness of PAN.

## Related Work

Fine-grained entity typing aims to assign entity mentions with a larger set of fine-grained types (Ling and Weld 2012), and has been paid great attention recent years. Unlike coarse entity typing (e.g., “person”, “location”), this task can not be tackled by multi-class classification following the type mutual exclusion assumption (i.e., one type per mention). Actually, it is formulated as multi-label multi-class classification problems, and type hierarchy is distinct in fine-grained entity typing.

A main challenge in fine-grained entity typing is the absence of annotated data, and the training data is generated by distant supervision. It uses a knowledge base to generate candidate types, and will inevitably introduce label noise. This problem is first discussed by (Gillick et al. 2014), which also introduces the concept of context-dependent fine-grained entity typing, where the types of a mention is constrained to what can be deduced from its context. In order to encourage more research on the problem, they introduce a new OntoNotes-derived manually annotated evaluation dataset. In addition, they proposed three label cleaning heuristics to reduce the label noise. However, using heuristics to prune wrong data will aggressively filter training examples, and may suffer from low recall (Ren et al. 2016). Therefore, (Ren et al. 2016) proposed a heterogeneous partial-label embedding framework to denoise candidate types by constituting a graph of entity mentions, context features and entity types, and jointly learning their embeddings. Nevertheless, the denoising process and the training process are not unified, which may lead to error propagation. In addition, they need to learn additional parameters apart from the training process, and their model complexity is proportional to the number of the features of the dataset and the edges in the graph.

Similar noise issue has also been encountered in relation extraction task, and the noise induced by distant supervision limit the accuracy of relation prediction. MultiR(Hoffmann et al. 2011) reduces the noise in the training data by selecting the most relevant sentence for each label while training. However, it do not make full use of the training data, and may limit the model performance. Inspired by this, (Lin et al. 2016) proposed a selective attention model to learn attention weights to score how well a sentence matches the relation and uses the weights to sum the sentences. It can avoid losing too much information and de-emphasize irrelevant sentences to reduce noise.

Inspired by their work, we propose our end-to-end path-based attention neural model to tackle the noise issue in fine-grained entity typing. We extend the denoise model in relation extraction to fine-grained typing, by considering the distinct hierarchical structure of types in this task. In this way, the noise can be reduced through an end-to-end process. As far as we know, we are the first to reduce noise in fine-grained entity typing through an attention based neural model by leveraging hierarchical structure of types.

## Path-Based Attention Neural Model

The architecture of PAN is illustrated in Figure2. Supposing that there are  $n$  sentences containing entity  $e$ , i.e.,  $\mathcal{S}_e = \{s_1, s_2, \dots, s_n\}$ , and  $\mathcal{T}_e$  is the automatically labeled types based on KBs. Firstly PAN employs LSTM to generate representations of sentences  $s_i$  following (Shimaoka et al. 2016), where  $s_i \in \mathbb{R}^d$  is the semantic representation of  $s_i$ ,  $i \in \{1, 2, \dots, n\}$ . Afterwards, we build path-based attention  $\alpha_{i,t}$  over sentences  $s_i$  for each type  $t \in \mathcal{T}_e$ , which is expected to focus on relevant sentences to type  $t$ . Then, the representation of sentence set  $\mathcal{S}_e$  for type  $t$ , denoted by  $s_{e,t} \in \mathbb{R}^d$ , is calculated through weighted sum of vectors of sentences. Finally, we obtain predicted types through a classification layer.

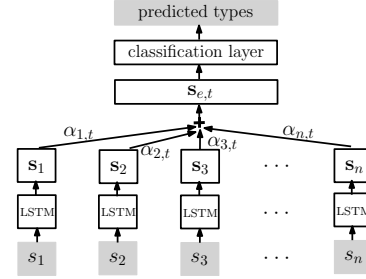

Figure 2: The architecture of PAN for given entity  $e$ , type  $t$

More precisely, given  $e$ , an attention  $\alpha_{i,t}$  is learned to score how well sentence  $s_i$  matches type  $t$ , i.e.,

$$\alpha_{i,t} = \frac{\exp(s_i \mathbf{A} \mathbf{p}_t)}{\sum_{j=1}^n \exp(s_j \mathbf{A} \mathbf{p}_t)},$$

where  $\mathbf{A} \in \mathbb{R}^{d \times d}$  is a weighted diagonal matrix.  $s_i \in \mathbb{R}^d$  is generated through an LSTM based neural model, and its architecture is illustrated in Figure3. Its input is the entity mention and context, and the output is the concatenation of entity mention representation and the context representation.

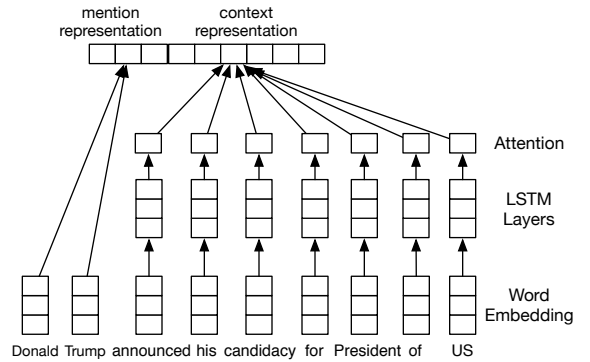

Figure 3: The distant supervision procedure to generate training data of “Donald Trump”.

In addition,  $\mathbf{p}_t \in \mathbb{R}^d$  is the representation of path  $p_t$  for type  $t$ . Specifically, for each type, we define one path

as a sequence of types starting from its coarsest parent type, and ending with it. More formally, for type  $t_l$ ,  $p_{t_l} = t_1 \rightarrow t_2 \rightarrow \dots \rightarrow t_l$ , where  $t_1$  is its coarsest parent type, and  $t_{i+1}$  is the subtype of  $t_i$ . For example, for type  $t_l = \text{politician}$ , its path is  $p_{t_l} = \text{person} \rightarrow \text{politician}$ . We represent the path  $p_{t_l}$  as a semantic composition of all the types on the path, i.e.,  $\mathbf{p}_{t_l} = \mathbf{t}_1 \circ \mathbf{t}_2 \circ \dots \circ \mathbf{t}_l$ , where  $\mathbf{t}_i \in \mathbb{R}^d$  is the representation of type  $t_i$ , which is a parameter to learn.  $\circ$  is a composition operator. In this paper, we consider two types of operators: (1) Addition (PAN-A), where  $\mathbf{p}_{t_l}$  equals the sum of type vectors. (2) Multiplication (PAN-M), where  $\mathbf{p}_{t_l}$  equals the cumulative product of type vectors. In this way, path-based attention enables the model to share parameters between types in the same path. For example, the attention learned for “person” could assist the learning of the attention for “politician”. It makes learning easier especially for infrequent subtypes, which suffer from dearth of training data, since the attentions for these subtypes can get support from the attention for parent type.

Then, the representation of sentence set  $\mathcal{S}_e$  for type  $t$ , i.e.,  $\mathbf{s}_{e,t}$ , is calculated through weighted sum of sentence vectors,

$$\mathbf{s}_{e,t} = \sum_{i=1}^n \alpha_{i,t} \mathbf{s}_i.$$

Since one mention can have multiple types, we employ a classification layer consisting of  $N$  logistic classifiers, where  $N$  is the total number of types. Each classifier outputs the probability of respective type, i.e.,

$$P(t|\mathbf{s}_{e,t}) = \frac{\exp(\mathbf{w}_t^T \mathbf{s}_{e,t} + \mathbf{b}_t)}{1 + \exp(\mathbf{w}_t^T \mathbf{s}_{e,t} + \mathbf{b}_t)},$$

where  $\mathbf{w}_t, \mathbf{b}_t \in \mathbb{R}^d$  are the logistic regression parameters. Here we adopt logistic regression classifier since the superiority of logistic regression classifier in fine-grained entity typing has been proved in (Gillick et al. 2014). To optimize the model, a multi-type loss is defined according to the cross entropy as follows,

$$J = - \sum_e \sum_t [\mathbb{I}_t \ln P(t|\mathbf{s}_{e,t}) + (1 - \mathbb{I}_t) \ln(1 - P(t|\mathbf{s}_{e,t}))],$$

where  $\mathbb{I}_t$  is indicator function to indicate whether  $t$  is the annotated type of entity  $e$ , i.e.,  $t \in \mathcal{T}_e$ .

## Experiments

Experiments are carried on two widely used datasets OntoNotes and FIGER(GOLD), and the training dataset of OntoNotes is noisy compared to FIGER(GOLD) according to (Shimaoka et al. 2016). The statistics of the datasets are listed in Table1. During training process, we use “raw” noisy data provided by (Shimaoka et al. 2016).

Table 1: Statistics of the datasets.

| Datasets    | #Type | #Layer | #Context | #Train | #Test |
|-------------|-------|--------|----------|--------|-------|
| OntoNotes   | 89    | 3      | 143K     | 223K   | 8,963 |
| FIGER(GOLD) | 113   | 2      | 1.51M    | 2.69M  | 563   |

We employ Strict Accuracy (Acc), Loose Macro F1 (Ma-F1), and Loose Micro F1 (Mi-F1) as evaluation measures following (Shimaoka et al. 2016) and Ren2016Label. Specifically, let  $T$  denote evaluation set. For each mention  $m \in T$ , we denote its ground-truth types as  $t_m$  and the predicted types as  $\bar{t}_m$ .

- Strict: The prediction is considered correct if and only if  $t_m = \bar{t}_m$ :

$$\text{Accuracy}(\mathbf{Acc}) = \sum_{m \in T} \mathbb{I}\{t_m = \bar{t}_m\} / |T|$$

- Loose Macro: The Macro-Precision (Ma-P) and MacroRecall (Ma-R) are computed for each mention, then their F1 is computed .

$$\mathbf{Ma-P} = \frac{1}{|T|} \sum_{m \in T} |t_m \cap \bar{t}_m| / |\bar{t}_m|$$

$$\mathbf{Ma-R} = \frac{1}{|T|} \sum_{m \in T} |t_m \cap \bar{t}_m| / |t_m|$$

$$\mathbf{Ma-F1} = \frac{2 * \mathbf{Ma-P} * \mathbf{Ma-R}}{\mathbf{Ma-P} + \mathbf{Ma-R}}$$

- Loose Micro: The Micro-Precision (Mi-P) and MicroRecall (Mi-R) scores are averages over all mentions, then their F1 is computed.

$$\mathbf{Mi-P} = \frac{\sum_{m \in T} |t_m \cap \bar{t}_m|}{\sum_{m \in T} |\bar{t}_m|}$$

$$\mathbf{Mi-R} = \frac{\sum_{m \in T} |t_m \cap \bar{t}_m|}{\sum_{m \in T} |t_m|}$$

$$\mathbf{Mi-F1} = \frac{2 * \mathbf{Mi-P} * \mathbf{Mi-R}}{\mathbf{Mi-P} + \mathbf{Mi-R}}$$

The baselines are chosen from two aspects: (1) Predicting types in a unified process using raw noisy data, i.e., TLSTM (Shimaoka et al. 2016), and other methods shown in Table2. (2) Predicting types using clean data by denoising ahead, i.e., H\_PLE and F\_PLE (Ren et al. 2016). To prove the superiority of considering type hierarchy, we also directly apply the attention neural model in relation extraction (Lin et al. 2016) without using type hierarchy (AN). We obtain the optimal hyperparameters from preliminary experiments by evaluating model performance on the development sets. Concretely, the hidden-size of the LSTM was set to 100, and we used Adam as our optimization method with a learning rate of 0.001, a mini-batch size of 1000. In order to make a fair comparison between the performance of our path-based attention mechanism and the neural architecture of (Shimaoka et al. 2016), we use the same word embeddings to represent sentence as they use. The results of baselines are the best results reported in their papers.

We can observed from Table2 that:

(1) When using the same raw noisy data, PAN outperforms all methods on both data sets. TLSTM achieves the best performance among baselines, while PAN-A improve 4% in Strict Accuracy, which is the most sensitive measure to noise and the most difficult one to enhance. Thus, it proves the anti-noise ability of PAN.

Table 2: Performance on FIGER(GOLD) and OntoNotes

| Metric | OntoNotes   |             |             | FIGER(GOLD) |             |             |
|--------|-------------|-------------|-------------|-------------|-------------|-------------|
|        | Acc         | Ma-F1       | Mi-F1       | Acc         | Ma-F1       | Mi-F1       |
| HYENA  | 24.9        | 49.7        | 44.6        | 28.8        | 52.8        | 50.6        |
| FIGER  | 36.9        | 57.8        | 51.6        | 47.4        | 69.2        | 65.5        |
| TLSTM  | 50.8        | 70.1        | 64.9        | 59.7        | 79.0        | 75.4        |
| AN     | 52.3        | 71.7        | 65.2        | 60.0        | 79.5        | 75.9        |
| PAN-A  | <b>54.9</b> | <b>72.8</b> | <b>66.5</b> | <b>60.2</b> | <b>79.9</b> | <b>76.2</b> |
| PAN-M  | 53.0        | 71.9        | 65.3        | 60.0        | 79.4        | 76.0        |

(2) PAN performs better than AN, it can be easily understood that the attention learned in PAN utilizes the hierarchical structure to enable parameter sharing, therefore, the type hierarchy can help to enhance the typing performance.

(3) The improvements on OntoNotes are higher than FIGER(GOLD), because OntoNotes is more noisy, and the hierarchical structure in OntoNotes is more complex with more layers, which further demonstrates that path-based attention does well with type hierarchy, and proves the superiority of PAN in reducing noise for data sets with more noise.

(4) PAN-A achieves better performance than PAN-M, which shows that addition operator can better capture type hierarchy.

Table 3: Performance on FIGER(GOLD) and OntoNotes

| Metric | OntoNotes   |             |             | FIGER(GOLD) |             |             |
|--------|-------------|-------------|-------------|-------------|-------------|-------------|
|        | Acc         | Ma-F1       | Mi-F1       | Acc         | Ma-F1       | Mi-F1       |
| H_PLE  | 54.6        | 69.2        | 62.5        | 54.3        | 69.5        | 68.1        |
| F_PLE  | <b>57.2</b> | 71.5        | 66.1        | 59.9        | 76.3        | 74.9        |
| PAN-A  | 54.9        | <b>72.8</b> | <b>66.5</b> | <b>60.2</b> | <b>79.9</b> | <b>76.2</b> |

As shown in Table3, PAN using raw noisy data outperforms H\_PLE and F\_PLE using denoised data on Ma-F1 and Mi-F1. It makes sense that F\_PLE has higher Acc on OntoNotes since the noise is reduced before training, but it needs to learn additional parameters about mentions, contexts and types, i.e., the semantic representation of mentions, contexts and types, while PAN only needs to learn parameters of attention, i.e., the semantic representation of types and the diagonal matrix. Note that the number of mentions and contexts are far more than the number of types. Thus, PAN is more efficient to reduce noise.

## Conclusion and Future Work

In conclusion, PAN can reduce noise through an end-to-end process, and thus can achieve better typing performance without bring much complexity. Moreover, it performs better on the dataset with more noise and more complex hierarchy. In the future, we will explore the formulation of path representations, such as using RNN or other operators to better capture the hierarchical constraints between types. Besides, we also think that we can better model the classification layer by considering type hierarchy, which may help to utilize the hierarchical structure more thoroughly.

## References

- Gillick, D.; Lazic, N.; Ganchev, K.; Kirchner, J.; and Huynh, D. 2014. Context-dependent fine-grained entity type tagging. *arXiv preprint arXiv:1412.1820*.
- Hoffmann, R.; Zhang, C.; Ling, X.; Zettlemoyer, L.; and Weld, D. S. 2011. Knowledge-based weak supervision for information extraction of overlapping relations. In *Proceedings of the 49th Annual Meeting of the Association for Computational Linguistics: Human Language Technologies-Volume 1*, 541–550. Association for Computational Linguistics.
- Lin, Y.; Shen, S.; Liu, Z.; and et al. 2016. Neural relation extraction with selective attention over instances. In *ACL*.
- Ling, X., and Weld, D. S. 2012. Fine-grained entity recognition. In *AAAI*.
- Ren, X.; He, W.; Qu, M.; Voss, C. R.; Ji, H.; and Han, J. 2016. Label noise reduction in entity typing by heterogeneous partial-label embedding. In *KDD*.
- Shimaoka, S.; Stenetorp, P.; Inui, K.; and Riedel, S. 2016. Neural architectures for fine-grained entity type classification. In *EACL*.
